# Supplementary material for: Nematic quantum phases in the bilayer honeycomb antiferromagnet
Source: arXiv:1712.08216 source file (2017-12-21)
Supplement: Supplementary file 1 [file supp-mat.pdf]

# Supplementary material - Nematic quantum phases in the bilayer honeycomb antiferromagnet

## I. SERIES EXPANSION

Here we provide some additional details about the series expansion results presented in the work. The dimer series expansion SE calculations start from the limit of isolated interlayer dimers coupled via $J_\perp$. For this we decompose the model Hamiltonian of Eq.(1) in the paper into

$$H = H_0 + V(J_1, J_2),$$

where $H_0$ represents decoupled interlayer dimers and $V(J_1, J_2)$ is the interaction part of the Hamiltonian, connecting dimers via on-layer nearest ($J_1$) and next-nearest ($J_2$) couplings in units of $J_\perp$ (see Fig. 1 in the paper).
The spectrum of $H_0$ is equidistant, which allows to organize the levels structure of $H_0$ in a block-diagonal form, being each block labeled by an energy quantum-number Q. In this way, Q=0 represents the ground state (*vacuum*), where all dimers are in the singlet state. Q=1 sector is composed by states obtained by creating one-triplet excitation (*particle*) on a given dimer, and so on. The cases in which $Q \geq 2$ represent multiparticle states and are not considered here.
The interacting part of the Hamiltonian $V(J_1, J_2)$ mixes different Q-sectors, losing $H$ the block diagonal structure of $H_0$. However it is possible to restore the block-diagonal form by application of continuous unitary transformations, using the flow equation method of Wegner[1]. The method can be applied perturbatively transforming $H$ onto an block-diagonal effective Hamiltonian $H_{\text{eff}}$, which has the structure

$$H_{\text{eff}} = H_0 + \sum_{n,m}^{\infty} c_{n,m} J_1^n J_2^m,$$

where $c_{n,m}$ are weighted products of terms in $V(J_1, J_2)$ which conserve the $Q$-number, whose weights are determined by recursive differential equations (see further details in Ref. 2).
The $Q$-number conservation allows the direct computation of several observables from $H_{\text{eff}}$ in terms of a SE in $J_1, J_2$. For the present model we have performed $O(4)$ SE in $J_1, J_2$ for ground state energy ($Q = 0$) and for the triplet dispersion $\omega$, *ie* $Q = 1$. Of particular interest for this work is the dispersion, since it allows to delimit the extension of the IDP phase. Note that the dispersion has two branches due to the presence of two dimers per unit cell in the honeycomb lattice. We refer for technical details about the calculation to ref.[2]. The complete expression for both branches of the dispersion $\omega_\pm(J_1, J_2)$ up to 4th order in $J_1, J_2$ has the following form

$$\omega_\pm(J_1, J_2) = \pm a(J_1, J_2) + b(J_1, J_2),$$

where

$$\begin{aligned}
a(J_1, J_2) = 8J_1\sqrt{3 + 2\cos(\alpha_x) + 2\cos(\alpha_x - \alpha_y) + 2\cos(\alpha_y)} \quad & | - 2J_1^3\cos(\alpha_x - \alpha_y) - 2J_1^3\cos(\alpha_y) + 7J_1^3 \\
& + J_2\left(5J_1^2 - 2J_1J_2 + 26J_2^2 - 6J_2\right)\cos(2\alpha_x) - 7J_1^2J_2\cos(\alpha_x - \alpha_y) + 5J_1^2J_2\cos(2(\alpha_x - \alpha_y)) + 10J_1^2J_2\cos(2\alpha_x - \alpha_y) \\
& + 10J_1^2J_2\cos(\alpha_x + \alpha_y) + 10J_1^2J_2\cos(\alpha_x - 2\alpha_y) - 7J_1^2J_2\cos(\alpha_y) + 5J_1^2J_2\cos(2\alpha_y) - 18J_1^2J_2 - 2J_1^2\cos(\alpha_x - \alpha_y) \\
& - 2J_1^2\cos(\alpha_y) + 6J_1^2 - \left(2J_1^3 + J_1^2(7J_2 + 2) + J_1J_2(9J_2 - 4) + J_2\left(3J_2^2 + 8J_2 - 8\right)\right)\cos(\alpha_x) - 9J_1J_2^2\cos(\alpha_x - \alpha_y) \\
& - 2J_1J_2^2\cos(2(\alpha_x - \alpha_y)) - 4J_1J_2^2\cos(2\alpha_x - \alpha_y) - 4J_1J_2^2\cos(\alpha_x + \alpha_y) - 4J_1J_2^2\cos(\alpha_x - 2\alpha_y) - 9J_1J_2^2\cos(\alpha_y) \\
& - 2J_1J_2^2\cos(2\alpha_y) + 19J_1J_2^2 + 4J_1J_2\cos(\alpha_x - \alpha_y) + 4J_1J_2\cos(\alpha_y) - 4J_1J_2 - 3J_2^3\cos(\alpha_x - \alpha_y) \\
& + 26J_2^3\cos(2(\alpha_x - \alpha_y)) + 5J_2^3\cos(3(\alpha_x - \alpha_y)) + 22J_2^3\cos(2\alpha_x - \alpha_y) + 15J_2^3\cos(3\alpha_x - \alpha_y) + 22J_2^3\cos(\alpha_x + \alpha_y) \\
& + 15J_2^3\cos(2\alpha_x + \alpha_y) + 15J_2^3\cos(\alpha_x + 2\alpha_y) + 22J_2^3\cos(\alpha_x - 2\alpha_y) + 15J_2^3\cos(3\alpha_x - 2\alpha_y) + 15J_2^3\cos(\alpha_x - 3\alpha_y) \\
& + 15J_2^3\cos(2\alpha_x - 3\alpha_y) + 5J_2^3\cos(3\alpha_x) - 3J_2^3\cos(\alpha_y) + 26J_2^3\cos(2\alpha_y) + 5J_2^3\cos(3\alpha_y) - 6J_2^3 - 8J_2^2\cos(\alpha_x - \alpha_y) \\
& - 6J_2^2\cos(2(\alpha_x - \alpha_y)) - 12J_2^2\cos(2\alpha_x - \alpha_y) - 12J_2^2\cos(\alpha_x + \alpha_y) - 12J_2^2\cos(\alpha_x - 2\alpha_y) - 8J_2^2\cos(\alpha_y) \\
& - 6J_2^2\cos(2\alpha_y) + 6J_2^2 + 8J_2\cos(\alpha_x - \alpha_y) + 8J_2\cos(\alpha_y) - 8|,
\end{aligned}$$

and

$$
\begin{aligned}
b(J_1,J_2) = 1 + \frac{1}{128}[&4\cos(\alpha_x)J_1^4 - 10\cos(2\alpha_x)J_1^4 + 4\cos(\alpha_x-\alpha_y)J_1^4 - 10\cos(2(\alpha_x-\alpha_y))J_1^4 - 20\cos(2\alpha_x-\alpha_y)J_1^4 \\
&+4\cos(\alpha_y)J_1^4 - 10\cos(2\alpha_y)J_1^4 - 20\cos(\alpha_x+\alpha_y)J_1^4 - 20\cos(\alpha_x-2\alpha_y)J_1^4 - 87J_1^4 - 432J_2J_1^3 \\
&+96J_2\cos(\alpha_x)J_1^3 - 32\cos(\alpha_x)J_1^3 + 32J_2\cos(2\alpha_x)J_1^3 + 96J_2\cos(\alpha_x-\alpha_y)J_1^3 - 32\cos(\alpha_x-\alpha_y)J_1^3 \\
&+32J_2\cos(2(\alpha_x-\alpha_y))J_1^3 + 64J_2\cos(2\alpha_x-\alpha_y)J_1^3 + 96J_2\cos(\alpha_y)J_1^3 - 32\cos(\alpha_y)J_1^3 + 32J_2\cos(2\alpha_y)J_1^3 \\
&+64J_2\cos(\alpha_x+\alpha_y)J_1^3 + 64J_2\cos(\alpha_x-2\alpha_y)J_1^3 + 72J_1^3 + 2988J_2^2J_1^2 - 720J_2J_1^2 + 92J_2^2\cos(\alpha_x)J_1^2 \\
&+64J_2\cos(\alpha_x)J_1^2 - 32\cos(\alpha_x)J_1^2 - 364J_2^2\cos(2\alpha_x)J_1^2 + 48J_2\cos(2\alpha_x)J_1^2 - 60J_2^2\cos(3\alpha_x)J_1^2 + 92J_2^2\cos(\alpha_x-\alpha_y)J_1^2 \\
&+64J_2\cos(\alpha_x-\alpha_y)J_1^2 - 32\cos(\alpha_x-\alpha_y)J_1^2 - 364J_2^2\cos(2(\alpha_x-\alpha_y))J_1^2 + 48J_2\cos(2(\alpha_x-\alpha_y))J_1^2 \\
&-60J_2^2\cos(3(\alpha_x-\alpha_y))J_1^2 - 368J_2^2\cos(2\alpha_x-\alpha_y)J_1^2 + 96J_2\cos(2\alpha_x-\alpha_y)J_1^2 - 180J_2^2\cos(3\alpha_x-\alpha_y)J_1^2 \\
&+92J_2^2\cos(\alpha_y)J_1^2 + 64J_2\cos(\alpha_y)J_1^2 - 32\cos(\alpha_y)J_1^2 - 364J_2^2\cos(2\alpha_y)J_1^2 + 48J_2\cos(2\alpha_y)J_1^2 - 60J_2^2\cos(3\alpha_y)J_1^2 \\
&-368J_2^2\cos(\alpha_x+\alpha_y)J_1^2 + 96J_2\cos(\alpha_x+\alpha_y)J_1^2 - 180J_2^2\cos(2\alpha_x+\alpha_y)J_1^2 - 180J_2^2\cos(\alpha_x+2\alpha_y)J_1^2 \\
&-368J_2^2\cos(\alpha_x-2\alpha_y)J_1^2 + 96J_2\cos(\alpha_x-2\alpha_y)J_1^2 - 180J_2^2\cos(3\alpha_x-2\alpha_y)J_1^2 - 180J_2^2\cos(\alpha_x-3\alpha_y)J_1^2 \\
&-180J_2^2\cos(2\alpha_x-3\alpha_y)J_1^2 + 144J_1^2 - 54J_2^4 - 336J_2^3 + 288J_2^2 + 168J_2^4\cos(\alpha_x) - 128J_2^3\cos(\alpha_x) - 64J_2^2\cos(\alpha_x) \\
&+128J_2\cos(\alpha_x) + 16J_2^4\cos(2\alpha_x) + 64J_2^3\cos(2\alpha_x) - 32J_2^2\cos(2\alpha_x) - 104J_2^4\cos(3\alpha_x) \\
&+16J_2^3\cos(3\alpha_x) - 10J_2^4\cos(4\alpha_x) + 168J_2^4\cos(\alpha_x-\alpha_y) - 128J_2^3\cos(\alpha_x-\alpha_y) - 64J_2^2\cos(\alpha_x-\alpha_y) \\
&+128J_2\cos(\alpha_x-\alpha_y) + 16J_2^4\cos(2(\alpha_x-\alpha_y)) + 64J_2^3\cos(2(\alpha_x-\alpha_y)) - 32J_2^2\cos(2(\alpha_x-\alpha_y)) \\
&-104J_2^4\cos(3(\alpha_x-\alpha_y)) + 16J_2^3\cos(3(\alpha_x-\alpha_y)) - 10J_2^4\cos(4(\alpha_x-\alpha_y)) + 136J_2^4\cos(2\alpha_x-\alpha_y) \\
&+32J_2^3\cos(2\alpha_x-\alpha_y) - 64J_2^2\cos(2\alpha_x-\alpha_y) - 112J_2^4\cos(3\alpha_x-\alpha_y) + 48J_2^3\cos(3\alpha_x-\alpha_y) \\
&-40J_2^4\cos(4\alpha_x-\alpha_y) + 168J_2^4\cos(\alpha_y) - 128J_2^3\cos(\alpha_y) - 64J_2^2\cos(\alpha_y) + 128J_2\cos(\alpha_y) + 16J_2^4\cos(2\alpha_y) \\
&+64J_2^3\cos(2\alpha_y) - 32J_2^2\cos(2\alpha_y) - 104J_2^4\cos(3\alpha_y) + 16J_2^3\cos(3\alpha_y) - 10J_2^4\cos(4\alpha_y) \\
&+136J_2^4\cos(\alpha_x+\alpha_y) + 32J_2^3\cos(\alpha_x+\alpha_y) - 64J_2^2\cos(\alpha_x+\alpha_y) - 60J_2^4\cos(2(\alpha_x+\alpha_y)) - 112J_2^4\cos(2\alpha_x+\alpha_y) \\
&+48J_2^3\cos(2\alpha_x+\alpha_y) - 40J_2^4\cos(3\alpha_x+\alpha_y) - 112J_2^4\cos(\alpha_x+2\alpha_y) + 48J_2^3\cos(\alpha_x+2\alpha_y) + 136J_2^4\cos(\alpha_x-2\alpha_y) \\
&+32J_2^3\cos(\alpha_x-2\alpha_y) - 64J_2^2\cos(\alpha_x-2\alpha_y) - 60J_2^4\cos(2(\alpha_x-2\alpha_y)) - 112J_2^4\cos(3\alpha_x-2\alpha_y) \\
&+48J_2^3\cos(3\alpha_x-2\alpha_y) - 60J_2^4\cos(4\alpha_x-2\alpha_y) - 112J_2^4\cos(\alpha_x-3\alpha_y) + 48J_2^3\cos(\alpha_x-3\alpha_y) - 112J_2^4\cos(2\alpha_x-3\alpha_y) \\
&+48J_2^3\cos(2\alpha_x-3\alpha_y) - 40J_2^4\cos(4\alpha_x-3\alpha_y) - 40J_2^4\cos(\alpha_x-4\alpha_y) - 40J_2^4\cos(3\alpha_x-4\alpha_y) - 40J2^4\cos(\alpha_x+3\alpha_y)],
\end{aligned}
$$

in which the $\alpha's$ are related with the $k$ reciprocal lattice vectors by $\alpha_x = \frac{\sqrt{3}}{2}k_x + \frac{3}{2}k_y$ and $\alpha_y = -\frac{\sqrt{3}}{2}k_x + \frac{3}{2}k_y$. The triplet gap $\Delta_\pm(J_1,J_2)$, that is, the minimum of the two dispersion branches $\omega_\pm(J_1,J_2)$ along the range presented in the work is given by

$$
\begin{aligned}
\Delta_\pm(J_1,J_2) = &-\frac{165J_1^4}{128} + \frac{9J_1^3J_2}{8} - \frac{3J_1^3}{16} - \frac{3J_1^2J_2^2}{2} - \frac{3J_1^2J_2}{4} + \frac{3J_1^2}{8} - \frac{33J_2^4}{8} - \frac{3J_2^3}{4} - \frac{3J_2^2}{2} + 3J_2 \\
&\pm\left| -\frac{3J_1^4}{16} - \frac{9J_1^3J_2}{8} + \frac{39J_1^2J_2^2}{8} - \frac{3J_1^2J_2}{2} - \frac{351J_1J_2^3}{8} + \frac{27J_1J_2^2}{2} - \frac{9J_1J_2}{2} + \frac{3J_1}{2}\right| + 1. \qquad (1)
\end{aligned}
$$

Finally, the critical line in the plane $J_2 - J_\perp$ presented in the figure 2A of the paper (dotted blue line) was then obtained by numerically solving $\Delta_\pm(1/J_\perp, J_2/J_\perp) = 0$, since that the unit in the paper is $J_1$ and not $J_\perp$ as presented here.

[1] F.J. Wegner, Ann. Phys. **3**, 77 (1994).
[2] C. Knetter and G.S. Uhrig, Eur. Phys. J. B **13**, 209 (2000).
